# Supplementary material for: Thermally driven two-magnet nano-oscillator with large spin-charge conversion
Source: arXiv:1909.12445 source file (2019-09-27)
Supplement: Supplementary file 1 [file supplemental.pdf]

# Supporting Information for: Thermally driven two-magnet nano-oscillator with large spin-charge conversion

Bassim Arkook,[†] Christopher Safranski,[‡] Rodolfo Rodriguez,[†] Ilya N. Krivorotov,[‡] Tobias Schneider,[¶] Kilian Lenz,[¶] Jürgen Lindner,[¶] Houchen Chang,[§] Mingzhong Wu,[§] Yaroslav Tserkovnyak,[‖] and Igor Barsukov[*,†]

†*Physics and Astronomy, University of California, Riverside, CA 92521*
‡*Physics and Astronomy, University of California, Irvine, CA 92697*
¶*Institute of Ion Beam Physics and Materials Research, Helmholtz-Zentrum Dresden - Rossendorf e.V., 01328 Dresden, Germany*
§*Department of Physics, Colorado State University, Fort Collins, CO 80523*
‖*Physics and Astronomy, University of California, Los Angeles, CA 90095*

E-mail: igorb@ucr.edu

# References

(1) Vansteenkiste, A.; Leliaert, J.; Dvornik, M.; Helsen, M.; Garcia-Sanchez, F.; Van Waeyenberge, B. The design and verification of MuMax3. *AIP Adv.* **2014**, *4*, 107133.

(2) Hirsch, J. E. Spin Hall Effect. *Phys. Rev. Lett.* **1999**, *83*, 1834–1837.

(3) Dyakonov, M. I. Spin Hall Effect. Spintronics. 2008; p 105.

(4) Sinova, J.; Valenzuela, S. O.; Wunderlich, J.; Back, C. H.; Jungwirth, T. Spin Hall effects. *Rev. Mod. Phys.* **2015**, *87*, 1213–1260.

(5) Taniguchi, T.; Grollier, J.; Stiles, M. D. Spin-Transfer Torques Generated by the Anomalous Hall Effect and Anisotropic Magnetoresistance. *Phys. Rev. Appl.* **2015**, *3*, 044001.

(6) Gibbons, J. D.; MacNeill, D.; Buhrman, R. A.; Ralph, D. C. Reorientable Spin Direction for Spin Current Produced by the Anomalous Hall Effect. *Phys. Rev. Appl.* **2018**, *9*, 064033.

(7) Das, K. S.; Liu, J.; van Wees, B. J.; Vera-Marun, I. J. Efficient Injection and Detection of Out-of-Plane Spins via the Anomalous Spin Hall Effect in Permalloy Nanowires. *Nano Lett.* **2018**, *18*, 5633–5639.

(8) Bose, A.; Lam, D. D.; Bhuktare, S.; Dutta, S.; Singh, H.; Jibiki, Y.; Goto, M.; Miwa, S.; Tulapurkar, A. A. Observation of Anomalous Spin Torque Generated by a Ferromagnet. *Phys. Rev. Appl.* **2018**, *9*, 064026.

(9) Safranski, C.; Montoya, E. A.; Krivorotov, I. N. Spin–orbit torque driven by a planar hall current. *Nat. Nanotech.* **2019**, *14*, 27.

(10) Davidson, A.; Amin, V. P.; Aljuaid, W. S.; Haney, P. M.; Fan, X. Perspectives of Electrically generated spin currents in ferromagnetic materials. *arXiv:1906.11772* **2019**,

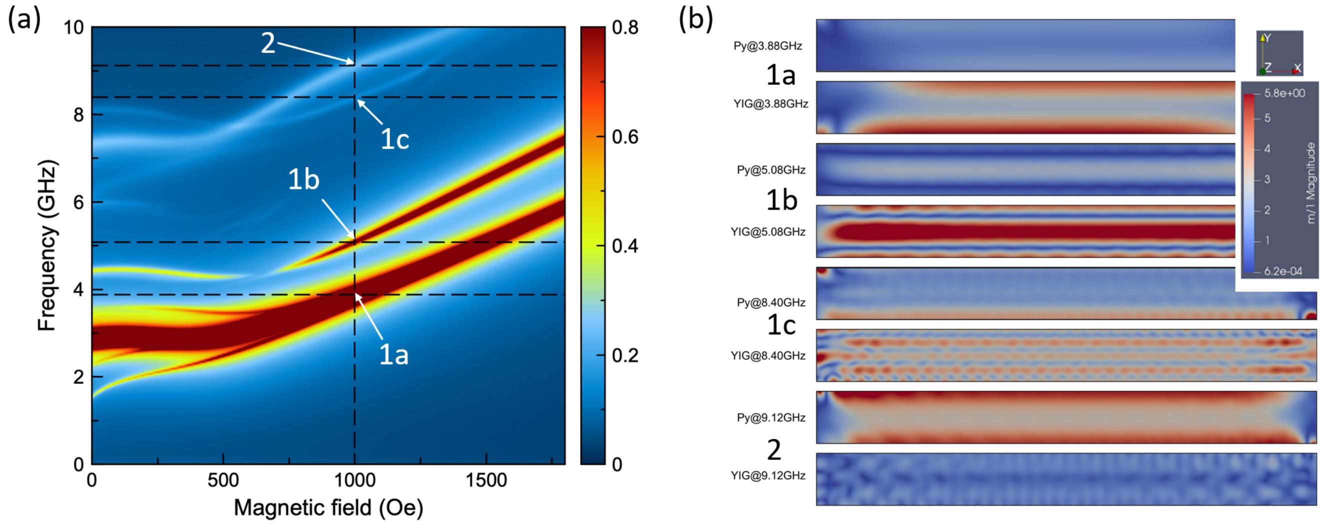


**Figure S1**: Micromagnetic simulations of YIG/Py nanowire using MuMax3 package.[1] Device geometry: length 3.8 nm, width 190 nm, YIG thickness 20 nm, Py thickness 5 nm. Cell size: 3.7 nm×5.9 nm×5.0 nm, temperature: 0 K, excitation by a sinc-pulse with lateral symmetry of 50 Oe (in z-direction). YIG magnetization 175 kA/m, Py magnetization 800 kA/m, YIG exchange constant $3.5\times10^{-12}$ J/m, Py exchange constant $13\times10^{-12}$ J/m. (a) Spatially averaged, normalized FFT of transverse components of magnetization is representative of excitation of spin waves close to hard-axis. Excitation magnitude is color-coded in arbitrary units. Modes '1a' and '1b' are excited in the experiment; mode '1c' is not sufficiently excited in the experiment. Mode '2' is sufficiently excited in short nanowires and in some of the long nanowires (supposedly due to symmetry-breaking defects present). (b) Lateral profile of excitations in YIG and Py layers for different frequencies at external field of 1000 Oe. With increasing frequency, delocalization and hybridization of spin waves increases. At low frequencies, the phase difference of magnetization precession between YIG and Py layer is nearly 0; at higher frequencies, the phase difference approaches $\pi$.

(11) Humphries, A. M.; Wang, T.; Edwards, E. R.; Allen, S. R.; Shaw, J. M.; Nembach, H. T.; Xiao, J. Q.; Silva, T. J.; Fan, X. Observation of spin-orbit effects with spin rotation symmetry. *Nat. Commun.* **2017**, *8*, 911.

(12) Safranski, C.; Barsukov, I.; Lee, H. K.; Schneider, T.; Jara, A.; Smith, A.; Chang, H.; Lenz, K.; Lindner, J.; Tserkovnyak, Y.; Wu, M.; Krivorotov, I. N. Spin caloritronic nano-oscillator. *Nat. Commun.* **2017**, *8*, 117.

| Spin-charge effect | Spin polarization $\vec{\sigma} \propto$ | Spin flow direction $\vec{I}_\sigma \propto$ | Damping/anti-damping character under field reversal | Anti-damping effect disappears when |
|---|---|---|---|---|
| Spin Hall[a] | $\vec{I}_e \times \vec{I}_\sigma$ | $\vec{I}_\sigma$ | odd | in easy-axis |
| Anomalous Hall[b] | $\vec{M}_{\mathrm{Py}}$ | $\vec{M}_{\mathrm{Py}} \times \vec{E}$ | odd | in easy-axis |
| 'Planar Hall' (AMR)[c] | $\vec{M}_{\mathrm{Py}}$ | $\vec{M}_{\mathrm{Py}}\,(\vec{M}_{\mathrm{Py}} \cdot \vec{E})$ | even | in film plane |
| Rotational-symmetry[d] | $\vec{\sigma}$ | $\vec{I}_e \times (\vec{M}_{\mathrm{Py}} \times \vec{\sigma})$ | even | $\vec{M}_{\mathrm{Py}} \,\|\|\, \vec{M}_{\mathrm{YIG}}$ collinear |

**Table S1**: Overview of some spin-orbit torques acting on YIG magnetization in the YIG/Py bilayer system, based on previous works. The damping-like torque considered here is exerted via an effective spin current. The spin current is described by the tensor product of spin polarization and spin flow direction $\vec{\sigma} \otimes \vec{I}_\sigma$. The spin current is generated in Py or at the interface. The damping/antidamping effect changes (odd) or maintains (even) sign under field reversal in the two-magnet nanowire (the field above remanence is assumed). The damping/antidamping effect vanishes for specific configurations of the magnetizations. a) Refs.;[2–4] b) Refs.;[5–8] c) Refs.;[5,9] d) Refs. [10,11]

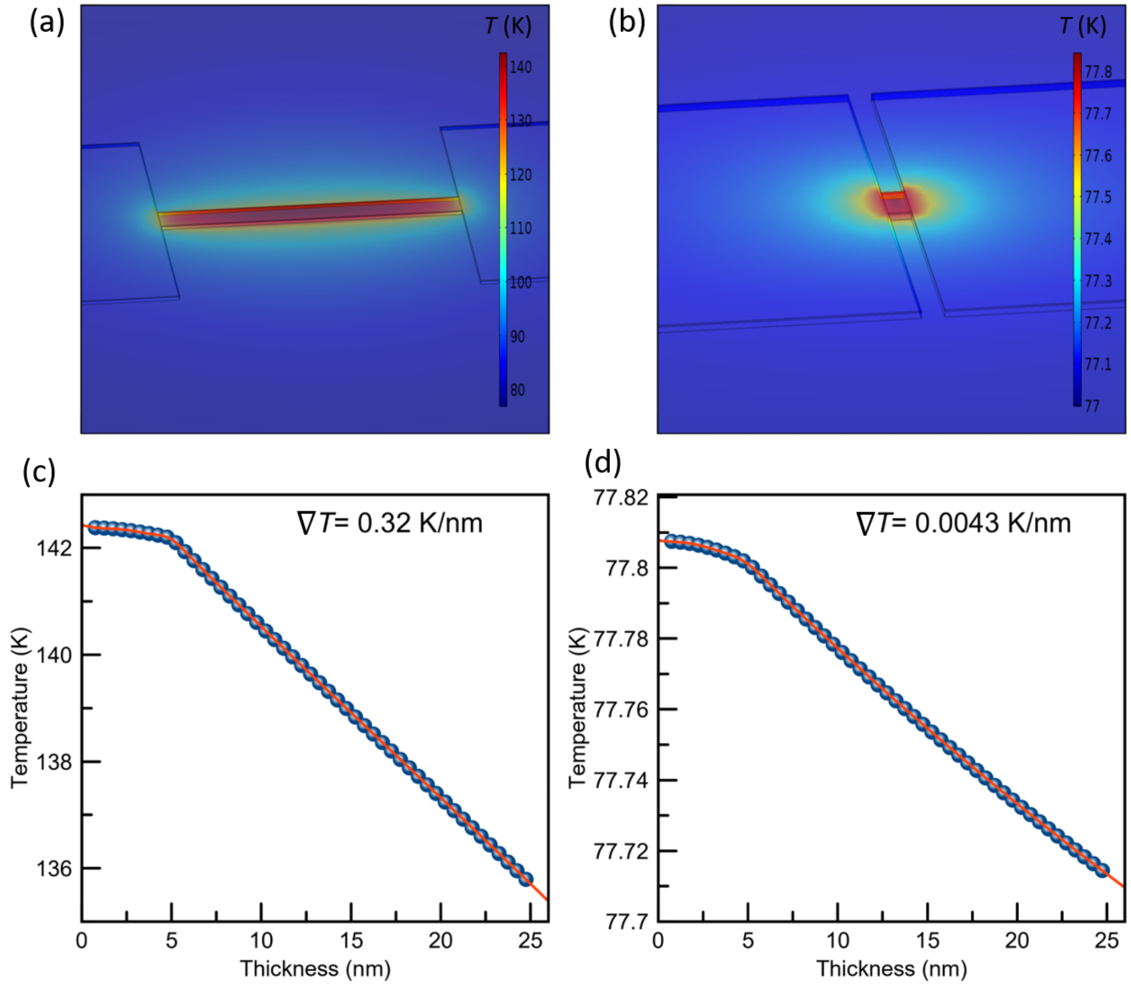


**Figure S2**: Finite-element simulation (in COMSOL Multiphysics) of temperature profile under ohmic heating of the Py layer. (a) Lateral profile of temperature (in Kelvin) of a long nanowire at $I$=1.87 mA. (b) Lateral profile of temperature (in Kelvin) of a short nanowire at $I$=1.66 mA. (c,d) Depth profiles of the temperature, counting the thickness from the top of the Py layer.

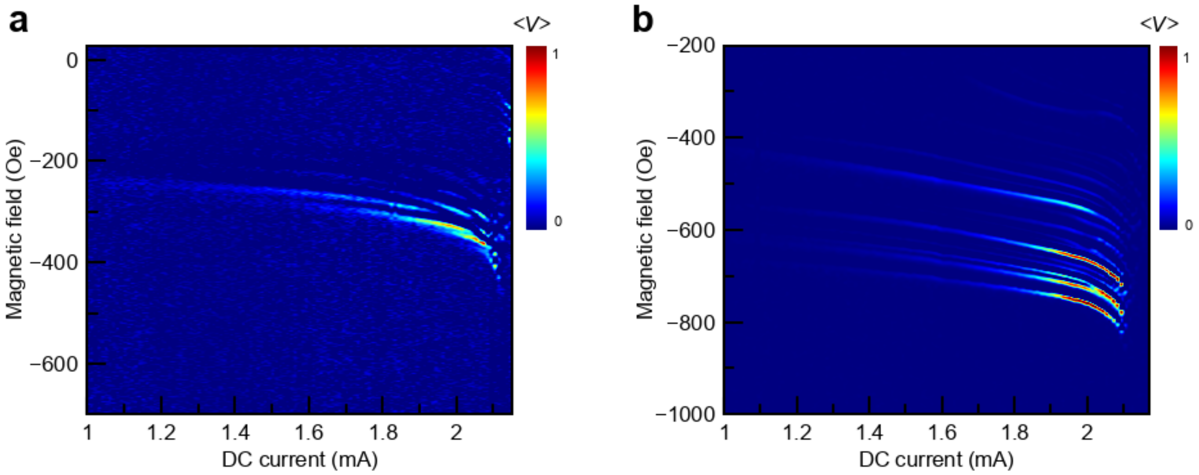


**Figure S3**: Microwave emission from the long nanowire at negative fields. The sample is wire-bonded to a co-planar waveguide, and the emitted microwave signal is passed through co-axial microwave cables to a bias-tee, pre-amplifier, and spectrum analyzer. The measurements are carried out using field modulation and single-frequency detection, as detailed in Ref. [12] (a) Easy-axis emission. (b) Hard-axis emission. The normalized detected voltage $\langle V \rangle$ is proportional to the spectral power density. Emission spectra very similar to those detected at positive external fields are observed.
